# Supplementary material for: Skeleton-Guided-Translation: A Benchmarking Framework for Code Repository Translation with Fine-Grained Quality Evaluation
Source: arXiv:2501.16050 source file (2025-01-27)
Supplement: Supplementary file 1 [file appendix.tex]

\appendix
\section{Appendix}
% The \FE~ and the \BE~ form a lens to maintain consistency between \textsl{source} (AST of programs with hole bindings) and \textsl{view} (output with hole closures). 

To ensure the stability of the system, the relationship of the \FE~ and the \BE~ should satisfy round-tripping properties, i.e., \GP~ and \WPG~ defined in Section \ref{sec:rtp}.

By induction on the evaluation derivation, \GP~ property can be easily proved. The proof of replacement and propagation rules is straightforward, but primitive rules especially division rules of integers need attention. For example, when the output value $2$ updates exact division expression $5//2$, some custom update rules use $4$ to update $5$, and the \GP~ law is not satisfied. Therefore, we check if the output value is the same as the original in primitive rules, and if so, the expression remains unchanged. The consistency check avoids spending meaningless time on updating the unchanged expression, which is an effective optimization in our approach.

The proof of the \WPG~ property is divided into two parts: the constraint backward evaluation is used to solve dependencies in programs; the second part proves that the three-way merge is correct in the constraint backward evaluation.

% The \PG~ property (not shown) requires that the modified program $\Sigma';E'\vdash e'$, obtained from the \BE~with the output value $v'$, can evaluate to just $v'$. The \PG~ property can be proved using the two-way merge which is an overly strict requirement in the present setting, particularly not applicable in programming with a lot of data dependencies. It is necessary to prove the property of bidirectional evaluation with the three-way merge, which does not satisfy \PG~but satisfies \WPG. 

\subsection{Constraint Backward Evaluation}
There are many data dependencies in the program, and a single primitive rule cannot solve all dependencies between sub-expressions, which leads to the dissatisfaction of \WPG.

\begin{example} Assume that the update strategy of plus is to ensure that the second expression remains unchanged and only modify the first expression. Consider the expression \verb|let x=1 in x+x|, which evaluates to $2$. If the output updates to $3$, the rules U-Let, U-Plus, and U-Var combine with the three-way merge to update the program to \verb|let x=2 in x+x|, which evaluates to $4$. However, if the output updates to $4$ directly, the original program will update to \verb|let x=3 in x+x|. \qed
\end{example}

Abstractly, the \BE~is a trade-off between efficiency and accuracy. In order to speed up the constraints-solving, we choose simplest primitive rules. In fact, constraint \BE~can solve the dependency more accurately, and here we use only the rule U-Plus as an example to show the definition.

\begin{align*}
\begin{array}{c}
r_1\;r_2\;are\;fresh\\
\Sigma;E\vdash e_1\Leftarrow r_1\leadsto \Sigma_1;E_1\vdash e_1'\vDash C_1\\
\Sigma;E\vdash e_2\Leftarrow r_2\leadsto \Sigma_2;E_2\vdash e_2'\vDash C_2\\
(E', C_E) = E_1\oplus E_2\quad (\Sigma', C_H)=\Sigma_1\oplus \Sigma_2 \\
C'=C_1 \cup C_2\cup \{r_1+r_2=r'\}\cup C_E\cup C_H\\
\midrule
\Sigma;E\vdash e_1+e_2\Leftarrow r'\leadsto \Sigma';E'\vdash e_1'+e_2'\vDash C'
\end{array}
\end{align*}

In constraint \BE, the definition of values not only includes hole values and determinate values, but also variables $r$. The rule U-Plus says that, when the output value $r'$ updates $e_1+e_2$, two fresh variables $r_1$ and $r_2$ are generated to update $e_1$ and $e_2$ respectively and the sub derivations return constraints $C_1$ and $C_2$. In environments merge and hole bindings merge, the same variable establishes a equation constraint between two values in $C_E$ and $C_H$. The final constraints $C'$ is the union of the above five constraints sets. The correct updated program can be obtained by solving constraints set returned by the constraint \BE~. Regarding the problem of control flow, a similar method can be used to solve it, which is ignored here.

\subsection{Correctness}
\begin{figure}[htb]
\begin{center}
    \begin{minipage}{\linewidth}
    \begin{center}
    E-Dup
        $\begin{array}{c}
            \Sigma;E\vdash x\Rightarrow v\\
            \midrule
            \Sigma;E\vdash dup\;x\Rightarrow[v, v]
        \end{array}$
    \end{center}
    \end{minipage}
    \begin{minipage}{\linewidth}
    U-Dup
        $\begin{array}{c}
         \,\\
         \midrule
        \Sigma;E,x\mapsto v\vdash dup\;x\Leftarrow [v_1, v_2]\leadsto \Sigma;E,x\mapsto v_1\vdash dup\;x
        \end{array}$
    \end{minipage}
\end{center}
\caption{Semantics of Dup}
\label{dup}
\end{figure}

To simplify the problem, we assume there is only one constant in the program. To proof \WPG, we use $dup$ constructor to rewrite the program, which is equivalent to the three-way merge and the definition is shown in Figure \ref{dup}.

The $dup$ constructor is equivalent to a variable copy switch, and it copies the original variables and replace the same variable in sub-expressions with different new variables, wherever the environment is to be merged in the \BE. The rule E-Dup says that $dup\;x$ is actually a list of two elements, both of which are $v$, while the rule U-Dup merges $v_1$ and $v_2 $ depends on the domains and problems. Here is an example, the rule U-Dup says that when the output value is $[v_1, v_2]$, $v_1$ is always used to update the binding of $x$.

Transforming the program to the form that all dups are advanced to the highest level of AST does not affect the semantics of the program. For example,
\begin{center}
\begin{BVerbatim}
let t = 1 in 
    let x = t in
        x + t
\end{BVerbatim}
\end{center}
is transformed to 
\begin{center}
\begin{BVerbatim}
let t = 1 in 
    let [t1, t2] = dup t in 
        t1 + t2
\end{BVerbatim}
\end{center}

It is easy to prove that the expressions inside dups satisfy \PG. This is because there is no data dependency and the requirement of two-way merge is satisfied, which leads to the satisfaction of the \PG~\cite{Mayer_2018}. 

Now we only need to prove that the part contains $dups$ satisfy \WPG, so that the entire program satisfies \WPG. The $dups$ part can be regarded as a data dependency tree formed by replication of variables. For example, consider the following transformed program.

\begin{center}
\begin{BVerbatim}
let t = 1 in 
    let [t1, t2] = dup t in
        let [t3, t4] = dup t2 in 
            t1::t2::t3::[]
\end{BVerbatim}
\end{center}

\begin{figure}
    \centering
    \includegraphics[width=0.4\linewidth]{figures/dependency.png}
    \caption{Dependency of Variables}
    \label{dependency}
\end{figure}

The data dependency of the above program can be represented by the tree in Figure \ref{dependency}. Assume $t1$ evaluates to $v_1$, $t3$ evaluates to $v_3$, and $t4$ evaluates to $v_4$. In other words, the output of the program is $[v_1, v_3, v_4]$. According to U-Dup, the values of leaf nodes $t1$ propagates to t and the constant $1$ in the source program updates to $v_1$. Then, the updated program evaluates to $[v_1,v_1,v_1]$, which updates the original program to the same one updated by $[v_1, v_3, v_4]$.

In conclusion, the above informal proof shows that \WPG~ is satisfied under the conditions explained earlier.
